# Supplementary material for: ComplexCodeEval: A Benchmark for Evaluating Large Code Models on More Complex Code
Source: arXiv:2409.10280 source file (2024-09-16)
Supplement: Supplementary file 1 [file 1_ComplexCodeEval-details.tex]

\begin{figure}
    \centering
    \includegraphics[width=1\linewidth]{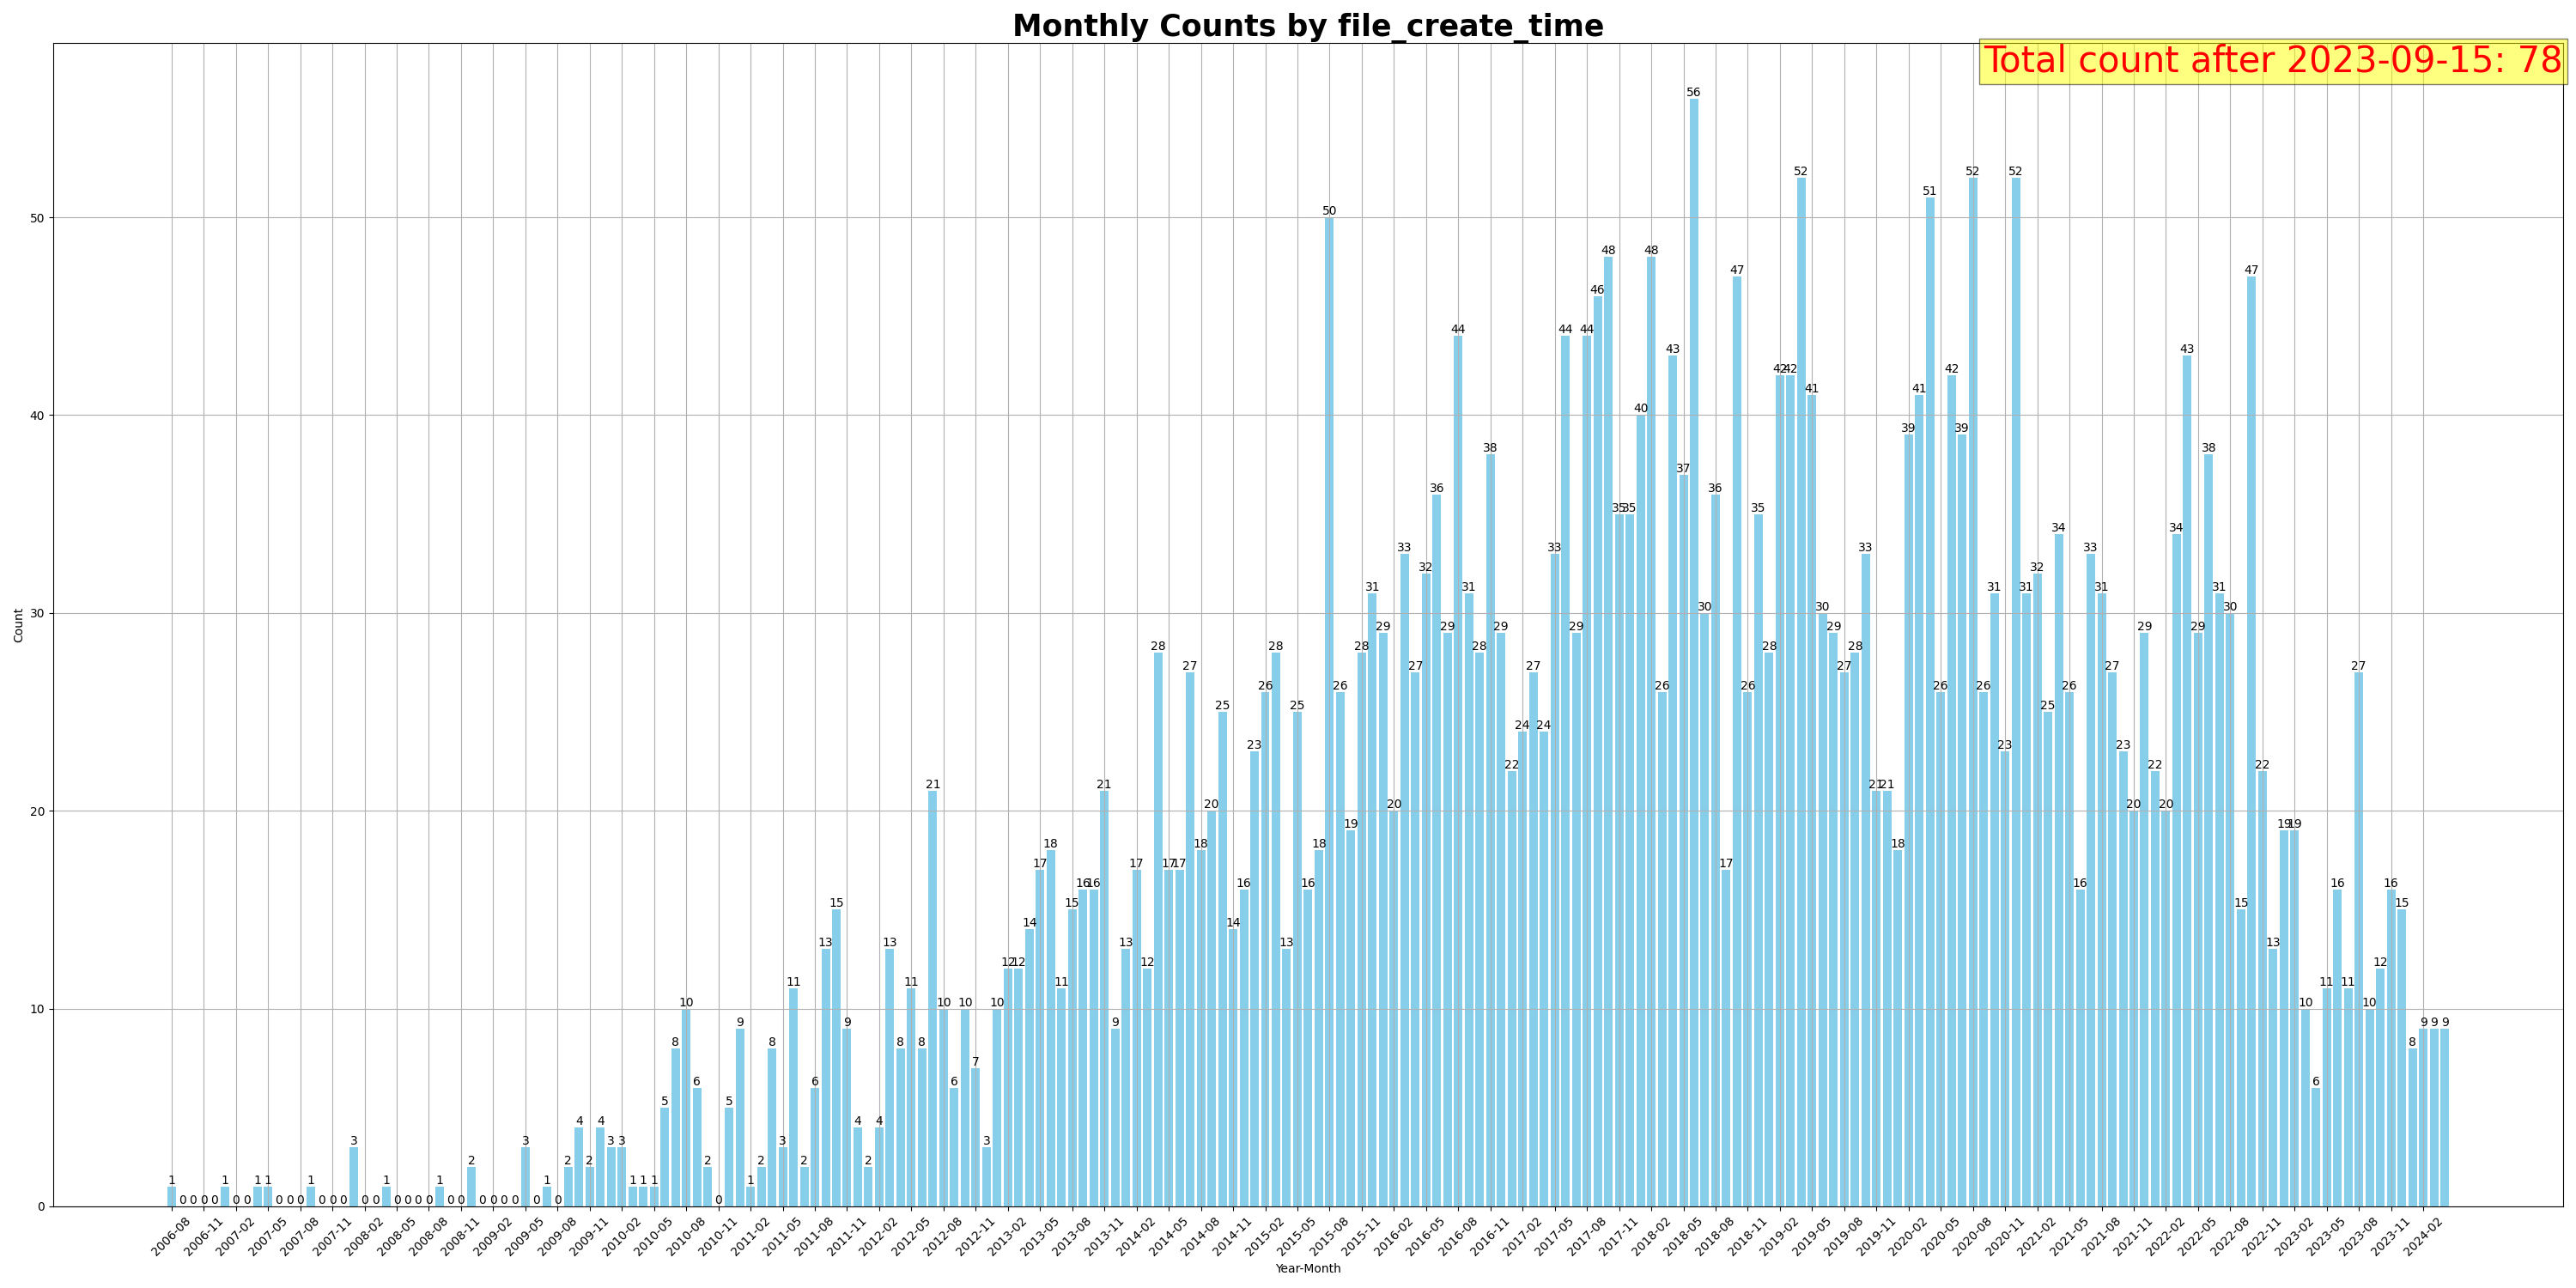}
    \caption{Distribution of File Creation Times in Java Data}
    \label{fig:file_create_time_Java}
\end{figure}
