# Supplementary material for: ComplexCodeEval: A Benchmark for Evaluating Large Code Models on More Complex Code
Source: arXiv:2409.10280 source file (2024-09-16)
Supplement: Supplementary file 2 [file 0_prompt-template.tex]

\begin{figure*}[t]
  \centering
  \begin{minipage}{\textwidth}
    \begin{tcolorbox}[width=\textwidth, colback=white]
      \begin{verbatim}
Here is the Java code:
'''Java
{code}
'''
Generate a Java Doc Comment for the Java code, which uses the API of {method}.
Generate the code comment in such a way that it is suitable to be used as a prompt for code generation.
Your response should only include the docstring, without explanation or formatting.
Here is an example of Java Doc Comment:
/**
 * Description: This method is for ... 
 * 
 * @param ... 
 * @param ... 
 * @return ... 
 */
      \end{verbatim}
    \end{tcolorbox}
    \captionsetup{justification=centering, width=\textwidth} 
    \caption{The prompt template for generating Java docstring with deepseekcoder.}
    \label{fig:java_prompt_template}
  \end{minipage}
\end{figure*}

\begin{figure}[t]
  \centering
  \begin{minipage}{\textwidth}
    \begin{tcolorbox}[width=\textwidth, colback=white]
      \begin{verbatim}
Here is the Python code:
'''Python
{code}
'''
Generate a Python Doc Comment for the Python code, which uses the API of {function}.
Generate the code comment in such a way that it is suitable to be used as a prompt for code generation.
Your response should only include the docstring, without explanation or formatting.
Here is an example of Python Doc Comment:
"""
Description: This function is for ...

Args:
    param1 (type): Description of param1    
    param2 (type): Description of param2    
    ...
    
Returns:
    type: Description of the return value
"""
      \end{verbatim}
    \end{tcolorbox}
    \captionsetup{justification=centering, width=\textwidth} 
    \caption{The prompt template for generating Python docstring with deepseekcoder.}
    \label{fig:python_prompt_template}
  \end{minipage}
\end{figure}
\clearpage
